# Supplementary material for: XPolicyLab: A Unified Standard and Open Ecosystem for Robot Policy Evaluation and Deployment
Source: arXiv:2608.09892 source file (2026-08-25)
Supplement: Supplementary file 1 [file appendix.tex]

\section*{APPENDIX}

Appendixes should appear before the acknowledgment.

\section*{ACKNOWLEDGMENT}
